# Supplementary material for: Weak formulation and spectral approximation of a Fokker-Planck equation for neural ensembles
Source: arXiv:2412.10676 source file (2024-12-14)
Supplement: Supplementary file 1 [file appendix.tex]

\appendix

\section{Appendix}
\label{sec:app}
\subsection{The basis functions of \texorpdfstring{$\mathrm{W}_1$}{} space}
\label{app:basis}
